# Supplementary material for: Slow rotation black hole perturbation theory
Source: arXiv:2305.19313 source file (2023-06-13)
Supplement: Supplementary file 1 [file supplemental_material.pdf]

# Slow rotation black hole perturbation theory - Supplemental Material

Nicola Franchini
*Université Paris Cité, CNRS, Astroparticule et Cosmologie, F-75013 Paris, France and CNRS-UCB International Research Laboratory, Centre Pierre Binétruy, IRL2007, CPB-IN2P3, Berkeley, CA 94720, USA*

## I. COEFFICIENTS OF THE PERTURBED EINSTEIN EQUATIONS

In this section, we provide the coefficients the appear in equations (11), (12a), (12b), (15a) and (15b). We start by showing all the coefficients of the first group

$$\begin{aligned}A^{(1)}_{0,\ell} =& \frac{H_2\rho^2}{2} + \frac{H_1\rho(3-4r)}{2r^2} - f_0\frac{H_0\ell(\ell+1)}{2r^2} + \frac{f_0(4r-1)H_0'}{4r^2} + f_0\frac{H_2'}{4r^2} + \frac{f_0^2H_0''}{2} - \rho f_0 H_1' - f_0\frac{K'}{2r^2} + K\rho^2 \\ &+ \frac{\mathrm{i}am(2r-1)H_1}{2r^5} + a^2\Bigg[\frac{H_0}{2r^4}\left(m^2 - \frac{1}{2f_0r^4} - \frac{2r^2+r-1}{r^3}\right) + \frac{H_2\left(2\rho^2r^4-6r+5\right)}{4f_0r^6} - \frac{\rho H_1'}{r^2} + \frac{f_0H_1\rho}{2r^4} \\ &+ \frac{\left(r^2+4r-1\right)H_0'}{4r^6} + \frac{H_2'}{2r^4} + \frac{f_0H_0''}{2r^2} - \frac{K'}{4r^4} - \frac{K\left(2\rho^2r^4-2r+1\right)}{4f_0r^6}\Bigg]\end{aligned} \tag{1a}$$

$$A^{(1)}_{1,\ell} = -a\frac{2h_0\ell(\ell+1)}{r^5} + \frac{\mathrm{i}ma^2}{r^5}\left[\frac{h_0\rho(r-2)}{f_0r} + f_0h_1' + \frac{h_1(8-7r)}{r^2}\right] \tag{1b}$$

$$\begin{aligned}A^{(1)}_{2,\ell} =& a^2\Bigg[-\frac{H_2\left(\rho^2r^4-7r+5\right)}{2r^6} + \frac{\rho f_0H_1'}{r^2} + \frac{H_1\rho\left(4r^2-6r+1\right)}{2r^5} + f_0H_0\left(\frac{\ell^2+\ell}{2r^4} + \frac{3}{4r^6}\right) \\ &- \frac{f_0\left(4r^2-10r+1\right)H_0'}{4r^5} - \frac{5f_0H_2'}{4r^4} - \frac{f_0^2H_0''}{2r^2} + \frac{(9r-10)K'}{4r^5} - \frac{K\left(2\rho^2r^5-4\rho^2r^4+14r^2-33r+20\right)}{4f_0r^7}\Bigg]\end{aligned} \tag{1c}$$

$$B^{(1)}_{1,\ell} = \frac{a}{2r^5}\left[-h_1\rho + (1-2r)h_0' - \frac{h_0(r-2)}{f_0r^2}\right] + \mathrm{i}ma^2\left[\frac{h_0\rho}{f_0r^4} - \frac{h_1}{2r^6}\right] \qquad B^{(1)}_{2,\ell} = \frac{a^2}{2r^5}\left[H_0\left(3-\frac{4}{r}\right) + H_2\right] \tag{1d}$$

$$\begin{aligned}A^{(2)}_{0,\ell} =& \frac{K\rho(2r-3)}{2r^2} - \frac{H_2\rho f_0}{r} - \frac{H_1f_0\ell(\ell+1)}{2r^2} + \rho f_0K' + \frac{\mathrm{i}ma}{2r^3}\left(\frac{H_0+H_2}{2r} - H_1\rho + f_0H_0'\right) \\ &+ \frac{a^2}{r^2}\left[H_1\left(\frac{m^2}{2r^2} - \frac{f_0}{r^3}\right) - \frac{3H_0\rho}{4r^3} + \frac{H_2\rho(1-2r)}{4r^2} - \frac{\rho K'}{2} + \frac{K\rho}{2f_0r^2}\right]\end{aligned} \tag{1e}$$

$$A^{(2)}_{1,\ell} = -a\frac{f_0h_1\ell(\ell+1)}{r^5} + \frac{\mathrm{i}ma^2}{r^4}\left(\frac{h_1\rho f_0}{r} - \frac{4h_0}{r^2} + f_0h_0'\right) \tag{1f}$$

$$A^{(2)}_{2,\ell} = \frac{a^2}{r^3}\left[\frac{3H_0\rho}{4r^2} + f_0H_1\frac{r\ell(\ell+1)+6}{2r^2} + H_2\rho\left(\frac{3}{2} - \frac{9}{4r}\right) + \rho\left(1-\frac{r}{2}\right)K' + \frac{3K\rho}{2r}\right] \tag{1g}$$

$$B^{(2)}_{1,\ell} = \frac{a}{r^3}\left[h_1\left(\frac{\rho^2}{2} - \frac{f_0}{r^2}\right) + \frac{h_0\rho}{r} - \frac{\rho h_0'}{2}\right] + \frac{\mathrm{i}ma^2}{2r^4}\left(h_1\rho - \frac{h_0}{f_0r^2} + h_0'\right) \qquad B^{(2)}_{2,\ell} = a^2f_0\frac{H_1(r+1)}{r^5} \tag{1h}$$

$$A^{(3)}_{0,\ell} = \frac{H_1\rho}{2r^2} - H_2\left(\frac{\rho^2}{2} + f_0\frac{\ell(\ell+1)}{2r^2}\right) - \frac{3f_0H_0'}{4r^2} - \frac{(4r-3)f_0H_2'}{4r^2} - \frac{f_0^2H_0''}{2} + \rho f_0 H_1' + \frac{(4r-3)f_0K'}{2r^2} + f_0^2K''$$
$$+ \frac{\mathrm{i}am}{r^3}\left(\frac{H_1}{2r^2} - H_2\rho + f_0H_1'\right) + \frac{a^2}{r^2}\Bigg[H_2\left(\frac{m^2}{2r^2} + \frac{2\left(\rho^2+4\right)r^2 - 10r + 3}{4f_0r^4}\right) - \frac{\rho H_1'}{r^2} + \frac{H_1\rho\left(-2r^3+r^2-1\right)}{2f_0r^4} - \frac{f_0H_2'}{2r}$$
$$+ \frac{\left(2r^3-r^2-8r+9\right)H_0'}{4r^4} + \frac{f_0H_0''}{2r^2} + \frac{H_0\left(22r^2-36r+15\right)}{4f_0r^6} + \frac{(3-4r)K'}{4r^2} - \frac{f_0K''}{2} - \frac{K\left(8r^2-10r+3\right)}{4f_0r^4}\Bigg] \tag{2a}$$

$$A^{(3)}_{1,\ell} = \frac{\mathrm{i}ma^2}{r^4}\left(h_0\rho + f_0^2h_1'\right) \tag{2b}$$

$$A^{(3)}_{2,\ell} = \frac{a^2}{r^3}\Bigg[H_1\rho\left(f_0 - \frac{1}{2r^2}\right) + H_2\left(\frac{\rho^2}{2} + f_0\frac{r\left(\ell^2+\ell-4\right)+3}{2r^2}\right) - \frac{f_0\left(2r^2+4r-9\right)H_0'}{4r^2} + \frac{f_0(6r-5)H_2'}{4r}$$
$$+ \frac{f_0^2H_0''}{2} + \frac{3f_0H_0(8r-5)}{4r^3} - \rho f_0H_1' + \frac{\left(4r^2-11r+6\right)K'}{4r^2} - \frac{f_0(r-2)K''}{2} + \frac{K\left(8r^3+2r^2-21r+12\right)}{4f_0r^4}\Bigg] \tag{2c}$$

$$B^{(3)}_{1,\ell} = \frac{a}{r^3}\left[\frac{h_1\rho}{2r^2} + \frac{(6r-5)h_0'}{2r^2} - \frac{h_0\left(12r^2-17r+6\right)}{2f_0r^4} + \rho f_0h_1' - f_0h_0''\right] + \frac{\mathrm{i}ma^2}{r^4}\left[\frac{h_1}{2r^2} + f_0h_1'\right] \tag{2d}$$

$$B^{(3)}_{2,\ell} = \frac{f_0a^2}{2r^4}\left(H_0 + 3H_2\right) \tag{2e}$$

$$A^{(4)}_{0,\ell} = \frac{H_0\ell(\ell+1)}{2r^2} - \frac{H_2\left(\ell^2+\ell+4\right)}{2r^2} - \frac{f_0\left(H_0'+H_2'\right)}{r} + \frac{2H_1\rho}{r} + \frac{(4r-3)K'}{r^2} + f_0K'' - K\left(\frac{\rho^2}{f_0} + \frac{\ell^2+\ell-2}{r^2}\right)$$
$$+ \frac{\mathrm{i}ma}{r^3}\left(\frac{2H_1}{r} - \frac{K\rho}{f_0}\right) + \frac{a^2}{r^2}\Bigg[\frac{\ell^2+\ell+2}{2f_0r^2}\left(K - \frac{H_0}{r^2} - H_2\right) + \frac{H_1\rho(4r+3)}{2r^2} + \frac{\left(3+r-4r^2\right)H_0'}{4r^3}$$
$$- \frac{\left(8r^2-r+1\right)H_2'}{4r^3} + \frac{H_0(2r+3)}{2r^4} - \frac{2H_2}{r^3} + \frac{\left(6r^2+r+1\right)K'}{2r^3} + K'' + K\left(\frac{3r-2}{f_0r^4} + \frac{\rho^2}{f_0^2r^2}\right)\Bigg] \tag{2f}$$

$$A^{(4)}_{1,\ell} = \frac{2ah_0\ell(\ell+1)}{(r-1)r^4} + \frac{2\mathrm{i}ma}{r^5}\left[\frac{2h_1\left(r^2-2r+2\right)}{r^2} - \frac{h_0\rho(r+1)}{f_0} + \left(r - \frac{1}{r}\right)h_1'\right] \tag{2g}$$

$$A^{(4)}_{2,\ell} = \frac{a^2}{r^2}\Bigg[\frac{r\left(\ell^2+\ell+6\right)+16}{2r^3}H_2 - \frac{H_1\rho(4r+3)}{2r^2} - \frac{r\left(\ell^2+\ell+12\right)+3}{2r^4}H_0 + \frac{f_0(4r+3)H_0'}{4r^2} + \frac{f_0(8r-1)H_2'}{4r^2}$$
$$+ \frac{\left(-6r^2+r-1\right)K'}{2r^3} - f_0K'' + \frac{K}{f_0}\left(\frac{r^2\left(\ell^2+\ell-6\right) - 2r\left(\ell^2+\ell+11\right)+20}{2r^4} + \frac{\rho^2}{r}\right)\Bigg] \tag{2h}$$

$$B^{(4)}_{1,\ell} = \frac{a}{r^4}\left[-h_1\rho + \frac{h_0\left(r\ell^2+r\ell+2\right)}{f_0r^2} + h_0'\right] - \frac{\mathrm{i}ah_1m}{r^6} \qquad B^{(4)}_{2,\ell} = \frac{a^2}{r^5}\left[H_0(-r-2) + H_2(2r+1) + \frac{K(2-4r)}{r-1}\right] \tag{2i}$$

then from the second group

$$\alpha^{(1)}_{0,\ell} = H_2\rho - \frac{H_1}{r^2} - f_0 H_1' + K\rho + \frac{a^2}{r^2}\left[\frac{H_1\left(2r^2-r+1\right)}{2r^3} + \frac{H_2\rho}{f_0} - H_1' - \frac{K\rho}{2f_0}\right] \tag{3a}$$

$$\alpha^{(1)}_{1,\ell} = \frac{a}{r^3}\left[\frac{h_1(7r-8)}{r^2} - 2f_0 h_1'\right] \qquad \alpha^{(1)}_{2,\ell} = \frac{a^2}{r^2}\left[-H_2\rho - \frac{H_1\left(2r^2-7r+1\right)}{2r^3} + f_0 H_1' - \frac{K\rho(r-2)}{2f_0 r}\right] \tag{3b}$$

$$\widetilde{\alpha}^{(1)}_{2,\ell} = \frac{a^2}{2r^2}\left[\frac{H_1\left(2r^2+r-1\right)}{r^3} - \frac{K\rho}{f_0}\right] \tag{3c}$$

$$\beta^{(1)}_{0,\ell} = \frac{2f_0 h_1\rho}{r} + \frac{h_0\left(r\ell^2+r\ell-2\right)}{r^3} + \rho f_0 h_1' - f_0 h_0'' \qquad \beta^{(1)}_{1,\ell} = \frac{a}{r^3}\left(H_2 - 2K\right) \tag{3d}$$

$$\beta^{(1)}_{2,\ell} = \frac{a^2}{r^2}\left[\frac{1+10r-4r^2}{2r^3}h_1\rho + \frac{2r^2\left(\ell^2+\ell+12\right) - r^3\ell(\ell+1) - 27r - 2}{2(r-1)r^4}h_0 - \frac{\left(2r^2+r+1\right)h_0'}{2r^3} - \rho f_0 h_1' + f_0 h_0''\right] \tag{3e}$$

$$\widetilde{\beta}^{(1)}_{2,\ell} = \frac{a^2}{2r^5}\left[h_1\rho + \frac{h_0\left(r^3(-\ell)(\ell+1) - 4r^2 + r - 2\right)}{(r-1)r} + \left(2r^2+r-1\right)h_0'\right] \tag{3f}$$

$$\eta^{(1)}_{1,\ell} = \frac{a h_1 \ell(\ell+1)}{2r^4} \qquad \eta^{(1)}_{2,\ell} = \frac{a^2}{r^2}\left[\frac{H_1(6r-8)}{r^3} + H_2\rho\left(\frac{1}{r}+1\right) - \frac{2K\rho}{r} - 2\frac{f_0 H_1'}{r}\right] \tag{3g}$$

$$\zeta^{(1)}_{1,\ell} = \frac{a}{r^2}\left[-2H_1\rho - \frac{H_0\ell(\ell+1)}{2r} + \frac{5f_0 H_0'}{2} - \frac{1}{2}f_0 H_2' + \frac{2H_2}{r} - \frac{K'}{r} + \frac{K\left(\rho^2 r^3 - 2r + 2\right)}{(r-1)r}\right] \tag{3h}$$

$$\zeta^{(1)}_{2,\ell} = \frac{a^2 h_0 (r-3)\ell(\ell+1)}{(r-1)r^5} \qquad \xi^{(1)}_{1,\ell} = \frac{aH_0}{2r^3} \qquad \xi^{(1)}_{2,\ell} = -\frac{a^2 h_0}{r^5} \qquad \chi^{(1)}_{1,\ell} = \frac{a}{r^3}\left(\frac{h_1}{2r} - \frac{h_0\rho}{f_0}\right) \tag{3i}$$

$$\alpha^{(2)}_{0,\ell} = H_1\rho + \frac{(H_0-H_2)(2r-3)}{2r^2} + \frac{H_2}{r^2} + f_0\left(K' - H_0'\right) + \frac{a^2}{r^3}\left[\frac{K(2r-1)}{2f_0 r} - \frac{3H_0}{2r^2} - \frac{H_1\rho}{f_0 r} + \frac{H_0'}{r} - \frac{(H_0+H_2)(2r+1)}{4r} - \frac{rK'}{2}\right] \tag{3j}$$

$$\alpha^{(2)}_{1,\ell} = \frac{a}{r^3}\left[-h_1\rho + \frac{h_0(8-9r)}{r-r^2} - h_0'\right] \tag{3k}$$

$$\alpha^{(2)}_{2,\ell} = \frac{a^2}{r^3}\left[-H_1\rho + \frac{H_0\left(-2r^2-5r+6\right)}{4r^2} + \frac{(r-1)H_0'}{r} + H_2\left(\frac{3}{2} - \frac{1}{4r}\right) + \left(1 - \frac{r}{2}\right)K' + \frac{K\left(2r^2-7r+4\right)}{2(r-1)r}\right] \tag{3l}$$

$$\widetilde{\alpha}^{(2)}_{2,\ell} = \frac{a^2}{r^2}\left[\frac{H_0\left(2r^2+r-6\right)}{4r^3} + \frac{H_2(2r+1)}{4r^2} - \frac{K'}{2}\right] \tag{3m}$$

$$\beta^{(2)}_{0,\ell} = h_1\left(\rho^2 + \frac{f_0\lambda}{r^2}\right) + \frac{2h_0\rho}{r} - \rho h_0' + \frac{a^2}{r^4}\left[\frac{h_0\rho\left(2r^2+r+4\right)}{2-2r} - h_1\left(\frac{\rho^2}{f_0} + \frac{f_0}{r} + \frac{\lambda+2}{2}\right) + \frac{\rho h_0'}{f_0}\right] \tag{3n}$$

$$\beta^{(2)}_{1,\ell} = \frac{aH_1}{r^3} \qquad \beta^{(2)}_{2,\ell} = \frac{a^2}{r^3}\left[\rho h_0' + \frac{h_0\rho\left(-2r^2+r+4\right)}{2(r-1)r} - h_1\left(\rho^2 + \frac{r^2\left(\ell^2+\ell-8\right) - 2r\left(\ell^2+\ell+1\right) + 10}{2r^3}\right)\right] \tag{3o}$$

$$\widetilde{\beta}^{(2)}_{2,\ell} = \frac{a^2}{r^4}\left[h_1\left(\frac{f_0}{r} - \frac{1}{2}\ell(\ell+1)\right) + h_0\rho\left(\frac{3}{2f_0} + r\right)\right] \qquad \eta^{(2)}_{1,\ell} = \frac{a\ell(\ell+1)}{2r^3}\left[3h_0' - 3h_1\rho + \frac{h_0(6-7r)}{(r-1)r}\right] \tag{3p}$$

$$\eta^{(2)}_{2,\ell} = \frac{a^2}{r^3}\left[\frac{H_0(8r-9)}{r^2} + 2H_1\rho r + \left(\frac{1}{r} - r\right)H_0' + H_2\left(\frac{1}{r} - 2\right) - 2K' + K\left(\frac{6}{r} + \frac{1}{r-1} + 2\right)\right] \tag{3q}$$

$$\zeta^{(2)}_{1,\ell} = \frac{a}{r}\left[\frac{3(H_0-H_2+2K)\rho}{2r} - \frac{H_1\ell(\ell+1)}{2r^2} + \rho K'\right] \qquad \zeta^{(2)}_{2,\ell} = -\frac{a^2 h_1 (r-2) f_0 \ell(\ell+1)}{r^5} \tag{3r}$$

$$\xi^{(2)}_{1,\ell} = \frac{aH_1}{2r^3} \qquad \xi^{(2)}_{2,\ell} = -\frac{a^2 h_1 f_0}{r^4} \qquad \chi^{(2)}_{1,\ell} = \frac{a}{r^3}\left[-h_1\rho + h_0\left(\frac{2}{r} + \frac{1}{r-1}\right) - h_0'\right] \tag{3s}$$

and finally from the third group

$$j_{0,\ell} = H_0 - H_2 - \frac{a^2}{f_0 r^2}\left(\frac{H_0}{r^2} + H_2\right) \qquad j_{2,\ell} = \frac{a^2}{r^2}\left(H_2 - \frac{H_0}{r}\right) \tag{4a}$$

$$k_{0,\ell} = 2\left(\frac{h_1}{r^2} - \frac{h_0\rho}{f_0} + f_0 h_1'\right) + \frac{2a^2}{r^2}\left[\frac{h_1(1-2r)}{2r^2} + \frac{h_0\rho}{f_0^2 r^2} + h_1'\right] \qquad k_{2,\ell} = \frac{2a^2}{r^3}\left[\frac{h_0\rho}{f_0} - f_0 r h_1' + h_1\left(1 - \frac{7}{2r}\right)\right] \tag{4b}$$

$$f_{1,\ell} = -\frac{2aK\rho}{f_0 r} \qquad f_{2,\ell} = \frac{4a^2}{r^3}\left[h_1\left(1 + \frac{7}{2r} - \frac{4}{r^2}\right) + \frac{h_0\rho}{f_0} - f_0 h_1'\right] \tag{4c}$$

$$g_{1,\ell} = \frac{3a}{r^2}\left[2h_0' - 2h_1\rho - h_0\left(\frac{2\ell(\ell+1)}{3f_0 r} + \frac{4}{r}\right)\right] \qquad g_{2,\ell} = \frac{2a^2}{r^2}\left[K\left(-\frac{2}{r} + \frac{1}{r-1} - 1\right) - H_2 f_0\right] \tag{4d}$$

$$h_{2,\ell} = \frac{a^2 h_1(2r+1)\ell(\ell+1)}{r^4} \tag{4e}$$

$$\widetilde{h}_{2,\ell} = \frac{a^2}{r^2}\left[\frac{H_0(9-2r)}{r^2} - H_1\rho + \frac{f_0(H_0' + H_2')}{2} - \frac{2H_2(r+2)}{r} + \left(4r + \frac{1}{r} + 1\right)K' - \frac{K\left(r^2\lambda + 4\right)}{f_0 r^2}\right] \tag{4f}$$

## II. DECOUPLING COEFFICIENTS

In this section we provide the decoupling coefficients that enter at second order in the spin in equations (36)-(39). We find it useful to define $\Gamma = (\lambda-4)(\lambda+2)r^2 + 6(\lambda+1)r + 9$ and $\Lambda = 3 + \lambda r$

$$\begin{aligned}
d_0^\ell = {} & 4\rho^2 \frac{3(\lambda-1) + (\lambda-4)(\lambda+2)r}{(5+4\lambda)\Gamma} + \frac{1}{(\lambda+2)(5+4\lambda)f_0\Gamma^2}\Bigg[-42\lambda^6 + 395\lambda^5 + 464\lambda^4 - 1240\lambda^3 - 8000\lambda^2 - 28976\lambda \\
& + \frac{27\left(13\lambda^3 - 125\lambda^2 + 290\lambda - 304\right)}{r^4} + \frac{9\left(43\lambda^4 - 260\lambda^3 + 597\lambda^2 - 1363\lambda - 2122\right)}{r^3} \\
& + \frac{3\left(47\lambda^5 - 483\lambda^4 + 485\lambda^3 - 1430\lambda^2 + 708\lambda + 10312\right)}{r^2} + \left(\lambda^2 - 2\lambda - 8\right)^2\left(29\lambda^2 + 53\lambda + 170\right)r \\
& + \frac{486(14-5\lambda)}{r^5} + \frac{17\lambda^6 - 428\lambda^5 + 1222\lambda^4 + 2856\lambda^3 + 10004\lambda^2 + 26084\lambda + 7144}{r} - 27968\Bigg] \\
& - 6f_0 m^2 \frac{(\lambda-16)r + 21}{(\lambda+2)^2\rho^2 r^7} + \rho^2 m^2 \frac{-6\left(2\lambda^2 + \lambda - 12\right) - 2(\lambda-4)(\lambda+2)(2\lambda+7)r}{(\lambda+2)^2(5+4\lambda)\Gamma} \\
& + \frac{m^2}{\Gamma^2}\Bigg[\frac{34\lambda^6 - 735\lambda^5 + 2940\lambda^4 + 7276\lambda^3 - 14592\lambda^2 + 10704\lambda + 39328}{2(\lambda+2)^2(4\lambda+5)} - \frac{486\left(19\lambda^2 + 33\lambda - 34\right)}{(\lambda+2)^3(4\lambda+5)r^4} \\
& + \frac{27\left(26\lambda^4 - 891\lambda^3 - 2190\lambda^2 + 216\lambda - 464\right)}{2(\lambda+2)^3(4\lambda+5)r^3} + \frac{9\left(86\lambda^5 - 1321\lambda^4 - 2146\lambda^3 + 6316\lambda^2 + 1072\lambda - 11216\right)}{2(\lambda+2)^3(4\lambda+5)r^2} \\
& + 2(\lambda+2)(\lambda-4)^2 r^2 - \frac{9\left(3\lambda^5 - 30\lambda^4 + 22\lambda^3 + 136\lambda^2 + 16\lambda + 960\right)r}{(\lambda+2)(4\lambda+5)} \\
& + \frac{3\left(94\lambda^6 - 1195\lambda^5 + 170\lambda^4 + 17688\lambda^3 + 19528\lambda^2 + 4960\lambda + 22016\right)}{2(\lambda+2)^3(4\lambda+5)r}\Bigg]
\end{aligned} \tag{5}$$

$$
\begin{aligned}
d_1^\ell = & \frac{1}{f_0^2(5+4\lambda)\Gamma}\Bigg[ -6\left(\lambda^3+\lambda^2+8\lambda-22\right) - \frac{18\left(2\lambda^2+3\lambda-14\right)}{(\lambda+2)r^3} - \frac{6\left(2\lambda^3+9\lambda^2-9\lambda+34\right)}{(\lambda+2)r^2} \\
& -2(\lambda+2)\left(\lambda^2+\lambda-20\right)r - \frac{18\left(\lambda^3+3\lambda^2+25\lambda+34\right)}{(\lambda+2)r}\Bigg] - \frac{18m^2}{(\lambda+2)^2\rho^2 r^5} \\
& \frac{m^2}{f_0(5+4\lambda)\Gamma}\Bigg[\frac{4\lambda^4-13\lambda^3+114\lambda^2+164\lambda-512}{(\lambda+2)^2} + \frac{-99\lambda^2+180\lambda+972}{(\lambda+2)^3 r^2} - 2\left(\lambda^2-14\lambda+40\right)r \\
& + \frac{6\left(2\lambda^4-7\lambda^3+24\lambda^2+184\lambda+148\right)}{(\lambda+2)^3 r}\Bigg]
\end{aligned}
\tag{6}
$$

$$
\begin{aligned}
d_K^\ell = & \frac{f_0}{r}d_H^\ell + \frac{\rho}{f_0\Lambda(5+4\lambda)}\Bigg[\frac{\lambda\left(\lambda^2+7\lambda+6\right)}{2r^2} - \frac{3\left(59\lambda^2-293\lambda+330\right)}{4(\lambda+2)r^6} + \frac{-11\lambda^3+488\lambda^2-1179\lambda+690}{(4\lambda+8)r^5} \\
& - \frac{\lambda\left(4\lambda^3+45\lambda^2-7\lambda+30\right)}{2(\lambda+2)r^3} + \frac{6\lambda^4+51\lambda^3-565\lambda^2+232\lambda-228}{4(\lambda+2)r^4} - \frac{72(\lambda-1)}{(\lambda+2)r^7}\Bigg] \\
& + \frac{m^2\rho}{\Lambda^2(5+4\lambda)}\Bigg[\frac{3\left(20\lambda^2+263\lambda+662\right)}{(\lambda+2)^3 r^6} + \frac{9\left(27\lambda^3+468\lambda^2+724\lambda-1264\right)}{4(\lambda+2)^3 r^5} + \frac{\lambda^2-3\lambda^3}{2r} \\
& + \frac{\lambda\left(25\lambda^4+596\lambda^3-554\lambda^2-5488\lambda-744\right)}{4(\lambda+2)^3 r^3} + \frac{61\lambda^4+1238\lambda^3+707\lambda^2-6272\lambda-108}{2(\lambda+2)^3 r^4} \\
& + \frac{\lambda\left(\lambda^5+15\lambda^4-143\lambda^3-514\lambda^2-148\lambda+24\right)}{2(\lambda+2)^3 r^2}\Bigg] - \frac{m^2}{\rho}\frac{\lambda(\lambda+4)r^2+3}{8(\lambda+2)r^9\Lambda^2}\left[(\lambda-2)\lambda r^2+(5\lambda-6)r+8\right]
\end{aligned}
\tag{7}
$$

$$
\begin{aligned}
d_H^\ell = {} & \frac{\rho^3}{f_0^2\Lambda(5+4\lambda)}\left[5(\lambda-5)+\frac{48}{\lambda+2}+\frac{24}{r^2}\left(\frac{3}{\lambda+2}-1\right)-2(2\lambda-3)r+\frac{3}{r}\left(15-3\lambda-\frac{40}{\lambda+2}\right)\right] \\
& + \frac{\rho}{f_0^2\Lambda^3(5+4\lambda)}\left[\frac{\left(56\lambda^3+197\lambda^2-244\lambda-60\right)\lambda^2}{2(\lambda+2)}-\frac{27\left(107\lambda^2-717\lambda+634\right)}{4(\lambda+2)r^5}\right. \\
& + \frac{3\left(44\lambda^3+4681\lambda^2-11139\lambda+8214\right)}{4(\lambda+2)r^4}+\frac{437\lambda^4+2395\lambda^3-21018\lambda^2+31950\lambda-11124}{4(\lambda+2)r^3} \\
& + \frac{80\lambda^5-561\lambda^4-4787\lambda^3+16494\lambda^2-9744\lambda+1440}{(4\lambda+8)r^2}-\frac{1080(\lambda-1)}{(\lambda+2)r^6}-\left(7\lambda^2+22\lambda+12\right)\lambda^2 r \\
& \left.+ \frac{\left(-39\lambda^4+11\lambda^3+1027\lambda^2-771\lambda+150\right)\lambda}{(\lambda+2)r}\right]-\frac{m^2\rho^3}{f_0\Lambda^3(5+4\lambda)(\lambda+2)}\left[2\lambda^2(2\lambda+1)r^3\right. \\
& + \frac{3\left(53\lambda^3-16\lambda^2-436\lambda+48\right)}{(\lambda+2)^2}+\frac{\lambda\left(7\lambda^4+28\lambda^3+72\lambda^2+160\lambda+48\right)r^2}{(\lambda+2)^2}+\frac{6\left(32\lambda^2+5\lambda-226\right)}{(\lambda+2)^2 r} \\
& \left.+ \frac{2\left(29\lambda^4+31\lambda^3-83\lambda^2+176\lambda+36\right)r}{(\lambda+2)^2}\right]+\frac{m^2\rho}{f_0\Lambda^4(5+4\lambda)(\lambda+2)}\left[\left(5\lambda^2+14\lambda-4\right)\lambda^3 r^2\right. \\
& + \frac{\left(4\lambda^5-349\lambda^4-2817\lambda^3+2792\lambda^2+21940\lambda+4944\right)\lambda^2}{2(\lambda+2)^2}+\frac{9\left(-28\lambda^2+899\lambda+2990\right)}{(\lambda+2)^2 r^5} \\
& + \frac{3\left(521\lambda^3+19916\lambda^2+24140\lambda-90288\right)}{4(\lambda+2)^2 r^4}+\frac{3\left(743\lambda^4+10952\lambda^3-22402\lambda^2-117840\lambda+58104\right)}{4(\lambda+2)^2 r^3} \\
& + \frac{3\left(247\lambda^5+1062\lambda^4-28714\lambda^3-52712\lambda^2+85688\lambda+2880\right)}{4(\lambda+2)^2 r^2} \\
& - \frac{\left(21\lambda^5+90\lambda^4-416\lambda^3-1540\lambda^2-624\lambda+48\right)\lambda^2 r}{(\lambda+2)^2} \\
& \left.+ \frac{\left(51\lambda^5-2508\lambda^4-34338\lambda^3-19904\lambda^2+149336\lambda+14400\right)\lambda}{4(\lambda+2)^2 r}\right]+\frac{m^2}{f_0\Lambda^5(\lambda+2)^2\rho}\left[\frac{135(7\lambda-34)}{r^8}\right. \\
& - \frac{\left(7\lambda^4-168\lambda^3-644\lambda^2+944\lambda+1536\right)\lambda^3}{8r^2}-\frac{3\left(163\lambda^3+86\lambda^2+1532\lambda-1032\right)\lambda}{4r^5} \\
& - \frac{\left(275\lambda^4+586\lambda^3-952\lambda^2-5856\lambda+1728\right)\lambda}{4r^4}-\frac{9\left(165\lambda^2+1876\lambda-3564\right)}{8r^7} \\
& - \frac{3\left(553\lambda^3-1236\lambda^2-2340\lambda+3024\right)}{8r^6}+\frac{-\frac{129\lambda^6}{8}+34\lambda^5+\frac{901\lambda^4}{2}+304\lambda^3-504\lambda^2}{r^3}+\frac{1728}{r^9} \\
& \left.+ \frac{\left(\lambda^3-3\lambda^2-34\lambda-24\right)\lambda^4}{r}\right]
\end{aligned} \tag{8}
$$

$$
\begin{aligned}
s_{1,0}^\ell = {} & 2\rho^4 r(\ell+3)\frac{r^2\ell\left(\ell^3+5\ell^2-\ell-21\right)-r\left(\ell^4+5\ell^3-2\ell^2-25\ell+21\right)-\ell^2-4\ell+21}{\ell(\ell+1)^4(\ell+2)(r\ell(\ell+3)+3)^2} \\
& + \rho^2(\ell+3)\frac{16r^3\ell^2(\ell+3)+r^2\ell\left(\ell^3-19\ell^2-57\ell+75\right)+r\left(-\ell^4+3\ell^3+14\ell^2-91\ell+27\right)-5\ell^2+16\ell-27}{2r^2\ell(\ell+1)^3(r\ell(\ell+3)+3)^2} \\
& + (\ell+2)\frac{2r^3\ell^2(\ell+3)^2-r^2\ell\left(2\ell^3+13\ell^2+16\ell-15\right)+r\left(\ell^3-2\ell^2-16\ell+3\right)+\ell-3}{4r^5(\ell+1)(r\ell(\ell+3)+3)^2}
\end{aligned} \tag{9}
$$

$$
\begin{aligned}
s_{1,1}^\ell = {} & \frac{r^2\ell^4+\left(3r^2+29r+8\right)\ell+r(5r+3)\ell^3+r(7r+20)\ell^2+20}{2r^3\ell(\ell+1)^2(r\ell(\ell+3)+3)} \\
& - \rho^2\frac{r\left(\ell^4+7\ell^3+9\ell^2-7\ell+6\right)+3\ell^2+14\ell-1}{\ell(\ell+1)^3(\ell+2)(r\ell(\ell+3)+3)}
\end{aligned} \tag{10}
$$

$$s^\ell_{1,K}=\frac{2f_0}{\ell+1}\left[4\rho^2\frac{\ell^3+7\ell^2+12\ell+2-r\left(\ell^3+5\ell^2+5\ell-3\right)}{r^4\ell(\ell+1)^2(\ell+2)}-\ell(\ell+3)\frac{r(\ell+2)-1}{r^7}+\frac{2\rho^4\left(\ell^3+5\ell^2-\ell-21\right)}{r\ell(\ell+1)^3(\ell+2)}\right] \tag{11}$$

$$\begin{aligned}s^\ell_{1,H}=&-\frac{(\ell+3)\left((r-1)r(r+3)\ell^2+r(r(r+4)-7)\ell-2r(r+2)+4\right)}{r^7(\ell+1)^2}+\frac{4\rho^4(\ell+3)(\ell(\ell+2)-7)}{\ell(\ell+1)^4(\ell+2)}\\&+\frac{\rho^2}{(\ell+1)^3}\left[\frac{\frac{6}{\ell}+2}{r^4}+\frac{2(\ell+3)(\ell(\ell(\ell(\ell+7)-3)-23)+2)}{r^2\ell(\ell+1)(\ell+2)}+\frac{2(\ell(\ell(\ell(3\ell+31)+103)+121)+14)}{r^3\ell(\ell+1)(\ell+2)}\right]\end{aligned} \tag{12}$$

$$\begin{aligned}t^\ell_{1,0}=&-2\rho^4r^3(\ell+3)\frac{r\ell^4+5r\ell^3-(r-1)\ell^2+(4-21r)\ell-21}{\ell(\ell+1)^4(\ell+2)(r\ell(\ell+3)+3)^2}\\&\frac{\rho^2}{(\ell+1)^3(\ell+1)(r\ell(\ell+3)+3)^2}\left[\frac{r^2\ell\left(\ell^3+5\ell^2-9\ell-29\right)(\ell+3)^2}{\ell+1}+\frac{3\left(5\ell+\frac{3}{\ell}+12\right)}{2r}\right.\\&\left.+\frac{r\left(\ell^6+5\ell^5+6\ell^4+18\ell^3+21\ell^2-231\ell-396\right)}{\ell+1}+\frac{17\ell^5+86\ell^4+154\ell^3+184\ell^2+21\ell-270}{2\ell(\ell+1)}\right]\\&+\frac{4r^3\ell^2(\ell+3)^2-2r^2\ell\left(\ell^3+7\ell^2+11\ell-3\right)+r\left(\ell^3+6\ell^2+11\ell-6\right)-3\ell+9}{4r^4(\ell+1)^2(r\ell(\ell+3)+3)^2}\end{aligned} \tag{13}$$

$$\begin{aligned}t^\ell_{1,1}=&2\rho^2r\frac{r\left(\ell^3+13\ell^2+31\ell+3\right)+\ell^2+8\ell+31}{f_0\ell(\ell+1)^4(\ell+2)(r\ell(\ell+3)+3)}\\&-\frac{r^2\left(4\ell^5+23\ell^4+27\ell^3-27\ell^2-35\ell+24\right)+4r^3\ell(\ell+1)^2(\ell+3)+r\left(17\ell^3+56\ell^2+7\ell-56\right)+12(\ell+1)}{2f_0r^3\ell(\ell+1)^3(\ell+2)(r\ell(\ell+3)+3)}\end{aligned} \tag{14}$$

$$t^\ell_{1,K}=2\rho^2(\ell+3)\frac{r\left(\ell^3+2\ell^2-7\ell-16\right)+6(\ell+2)}{r^3\ell(\ell+1)^3(\ell+2)}+12\frac{1-r(\ell+2)}{r^6(\ell+1)^2(\ell+2)} \tag{15}$$

$$\begin{aligned}t^\ell_{1,H}=&\frac{-2r^2\ell(\ell+2)(\ell+1)^2+r\left(2\ell^5+19\ell^4+56\ell^3+43\ell^2-16\ell+4\right)-\ell\left(\ell^3+6\ell^2-7\ell-36\right)}{(r-1)r^4\ell(\ell+1)^3(\ell+2)}\\&+2\rho^2(\ell+3)\frac{2r\left(\ell^2-6\ell-15\right)+\ell^2+6\ell+29}{(r-1)r\ell(\ell+1)^4(\ell+2)}\end{aligned} \tag{16}$$

$$u^\ell_0=\frac{2(\ell+3)(r(\ell+2)((2r-1)\ell(\ell+3)(\ell+4)+6)+3(\ell+1))}{r^3(\ell+1)^2(\ell+2)(r\ell(\ell+3)+3)}+\frac{\rho^2(\ell+3)(\ell+4)(\ell+9)}{2(\ell+1)^2(\ell+2)(2\ell+3)} \tag{17}$$

$$u^\ell_1=\frac{4(\ell+3)(\ell+4)}{(r-1)(\ell+1)^2(\ell+2)} \tag{18}$$

$$\begin{aligned}u^\ell_K=&\frac{r\left(2r^2(\ell+1)(\ell+3)(\ell+4)(4\ell+9)-r(\ell(\ell(2\ell(\ell+13)+99)+125)+26)+2\ell^2+\ell-21\right)+12}{2r^4(\ell+1)(\ell+2)(r(\ell+1)(\ell+4)+3)}\\&+\rho^2\frac{r(\ell+1)(\ell+3)(\ell+4)(\ell(\ell+9)+30)+\ell(\ell(3\ell+4)+19)+114}{2(\ell+1)^2(\ell+2)(2\ell+3)(r(\ell+1)(\ell+4)+3)}\end{aligned} \tag{19}$$

$$\begin{aligned}u^\ell_H=&\frac{\rho^2r^2(8r(\ell+3)(\ell+4)-11\ell-35)}{(r-1)(\ell+1)^2(\ell+2)(r(\ell+1)(\ell+4)+3)}\\&+\frac{1}{f_0(3+(\ell-3)\ell r)}\left[\frac{(\ell+4)\left(8\ell^2+41\ell+49\right)}{(\ell+1)(\ell+2)}-\frac{\left(4\ell^3+50\ell^2+182\ell+197\right)}{r(\ell^2+3\ell+2)}\right.\\&\left.+\frac{3(17\ell+41)}{4r^3(\ell+1)^2(\ell+2)}+\frac{7\ell^3+48\ell^2+74\ell-3}{r^2(\ell+1)^2(\ell+2)}\right]\end{aligned} \tag{20}$$

$$v_0^\ell = 2\rho^2 f_0(\ell+3)\frac{\ell(2r(\ell+3)(\ell+4)-\ell+1)+18}{r(\ell+1)^2(\ell+2)(r\ell(\ell+3)+3)} + f_0(\ell+3)\frac{8r^2\ell(\ell+3)(\ell+4)-2r\ell(\ell+3)(3\ell+17)+24r+\ell(5\ell+19)-18}{2r^4(\ell+1)(r\ell(\ell+3)+3)} \tag{21}$$

$$v_1^\ell = \frac{(5r-2)(\ell+3)(\ell+4)}{r^3(\ell+1)(\ell+2)} + \frac{\rho^2(\ell+3)(\ell+4)(\ell+9)}{2(\ell+1)^2(\ell+2)(2\ell+3)} \tag{22}$$

$$v_K^\ell = \rho^2 f_0 \frac{r(\ell+1)(\ell+3)(\ell+4)+11\ell+35}{r(\ell+1)^2(\ell+2)(r(\ell+1)(\ell+4)+3)} + f_0(\ell+3)\frac{r(\ell+1)(4\ell+7)(r(\ell+4)-1)-8}{2r^4(\ell+1)(r(\ell+1)(\ell+4)+3)} \tag{23}$$

$$v_H^\ell = \rho^2 \frac{r(\ell+3)(\ell+4)(\ell(\ell(\ell+14)+17)-12)+\ell(\ell(3\ell+92)+431)+534}{2(\ell+1)^2(\ell+2)(2\ell+3)(r(\ell+1)(\ell+4)+3)} - \frac{-2r^2(\ell+1)(\ell+3)(\ell+4)(9\ell+17)+2r(\ell+1)(\ell(\ell(5\ell+56)+180)+163)+\ell(19\ell+124)+153}{4r^3(\ell+1)^2(r(\ell+1)(\ell+4)+3)} \tag{24}$$
